# Supplementary material for: Boosting Flow-based Generative Super-Resolution Models via Learned Prior
Source: arXiv:2403.10988 source file (2024-05-29)
Supplement: Supplementary file 2 [file github.tex]

For assessing reproducibility, we provide the anonymous GitHub link of our project: \url{https://anonymous.4open.science/r/FlowSR-LP-6385/}
